# Supplementary material for: Modeling Student Performance in Game-Based Learning Environments
Source: arXiv:2309.13429 source file (2023-09-23)
Supplement: Supplementary file 1 [file appendix.tex]

\section{Appendix}
\label{sec:appendix}

To be filled.
